# Supplementary material for: Projected Topological Branes
Source: arXiv:2112.06911 ancillary file (2022-09-16)
Supplement: Supplementary file 1 [file PTB_Supplementary.pdf]

# Supplementary Information: Projected Topological Branes

Archisman Panigrahi,<sup>1,2</sup> Vladimir Jurić,<sup>3,4,\*</sup> and Bitan Roy<sup>2,5,†</sup>

<sup>1</sup>*Indian Institute of Science, Bangalore 560012, India*

<sup>2</sup>*Max-Planck-Institut für Physik komplexer Systeme, Nöthnitzer Str. 38, 01187 Dresden, Germany*

<sup>3</sup>*Nordita, KTH Royal Institute of Technology and Stockholm University,  
Hannes Alfvéns väg 12, SE-106 91 Stockholm, Sweden*

<sup>4</sup>*Departamento de Física, Universidad Técnica Federico Santa María, Casilla 110, Valparaíso, Chile*

<sup>5</sup>*Department of Physics, Lehigh University, Bethlehem, Pennsylvania, 18015, USA*

## CONTENTS

|                                                                                            |    |
|--------------------------------------------------------------------------------------------|----|
| Supplementary Note 1. Hamiltonian of the projected brane and its gap structure             | 1  |
| Supplementary Note 2. Chern Number of Model in Eq.(3) of the main text                     | 3  |
| A. Chern insulator and Chern number                                                        | 3  |
| B. Real space version of the spinless Bernevig-Hughes-Zhang Hamiltonian                    | 4  |
| C. Local Chern number ( $C_L$ ) on a square lattice                                        | 4  |
| D. Local Chern number of projected topological branes                                      | 5  |
| Supplementary Note 3. Real Space Hamiltonian with a single edge dislocation                | 5  |
| Supplementary Note 4. 3D Weyl semimetals: Lattice model, Landau levels, and chiral anomaly | 6  |
| A. Band structure of three-dimensional (3D) Weyl semimetals (WSMs)                         | 6  |
| B. Fermi Arc surface states of 3D Weyl semimetals                                          | 7  |
| C. 3D Landau levels with explicit form of Peierls factors                                  | 8  |
| D. Singular flux configuration and charge accumulation due to chiral anomaly               | 9  |
| Supplementary Note 5. Derivation of Eq.(5) of main text                                    | 10 |
| References                                                                                 | 11 |

## Supplementary Note 1. HAMILTONIAN OF THE PROJECTED BRANE AND ITS GAP STRUCTURE

We here present the derivation of Eq. (1) in the main text. The Hilbert space of the parent system is decomposed into two subsystems,  $\mathcal{H} = \mathcal{H}_1 \oplus \mathcal{H}_2$ , where the index 1 (2) corresponds to the subspace inside (outside) the brane. The parent Hamiltonian is given by Eq. (2) in the main text, which we here rewrite for completeness,

$$H_{\text{parent}} = \begin{pmatrix} H_{11} & H_{12} \\ H_{21} & H_{22} \end{pmatrix}, \quad (\text{S1})$$

and  $h = \sum \Psi^\dagger H_{\text{parent}} \Psi$ , with the spinor  $\Psi^\top = (\Psi_1, \Psi_2)^\top$  decomposed into the components acting in the two subspaces  $\mathcal{H}_1$  and  $\mathcal{H}_2$ . The sum over the internal indices within a Hilbert space is assumed. To integrate out the degrees of freedom outside the brane represented by the spinor  $\Psi_2$ , we write the imaginary-time partition function of the system as

$$\mathcal{Z} = \int \mathcal{D}\Psi \mathcal{D}\Psi^\dagger \exp \left\{ - \int d\tau \Psi^\dagger (\partial_\tau + H_{\text{parent}}) \Psi \right\} = \int \mathcal{D}\Psi_1 \mathcal{D}\Psi_1^\dagger \exp \left\{ - \int d\tau \Psi_1^\dagger (\partial_\tau + H_{11}) \Psi_1 \right\} \times \mathcal{I}(\Psi_1), \quad (\text{S2})$$

and the imaginary-time derivative acts on the right. Here, we define

$$\mathcal{I}(\Psi_1) = \int \mathcal{D}\Psi_2 \mathcal{D}\Psi_2^\dagger \exp \left\{ - \Psi_2^\dagger (\partial_\tau + H_{22}) \Psi_2 - \Psi_1^\dagger H_{12} \Psi_2 - \Psi_2^\dagger H_{21} \Psi_1 \right\}. \quad (\text{S3})$$

---

\* Corresponding author:juric@nordita.org

† Corresponding author:bitan.roy@lehigh.edu

The Greens's function reads as

$$\mathcal{G}(\tau) = (-\partial_\tau - H_{22})^{-1}, \quad (\text{S4})$$

or, alternatively, in terms of the (fermionic or bosonic) Matsubara frequency corresponding to the spinor  $\Psi_2$  assumes the form

$$\mathcal{G}(i\omega) = (i\omega - H_{22})^{-1}. \quad (\text{S5})$$

We also define the set of fields

$$\Phi = H_{21}\Psi_1, \quad \Phi^\dagger = \Psi_1^\dagger H_{12}, \quad (\text{S6})$$

where we used that  $H_{12} = H_{21}^\dagger$ . To carry out the integration in Eq. (S3), we introduce the new variables

$$\Psi'_2 = \Psi_2 - \mathcal{G}\Phi, \quad \Psi'^{\dagger}_2 = \Psi_2^\dagger - \Phi^\dagger \mathcal{G}, \quad (\text{S7})$$

with  $(\mathcal{G}\Phi)(\tau) \equiv \int d\tau' \mathcal{G}(\tau - \tau')\Phi(\tau')$ . After inserting the last equations into Eq. (S3) and integrating over  $\Psi_2$ , we find

$$\mathcal{I} = \mathcal{C} \exp \left\{ - \int d\tau d\tau' \Phi^\dagger(\tau) \mathcal{G}(\tau - \tau') \Phi(\tau') \right\} = \mathcal{C} \exp \left\{ - \int d\tau d\tau' \Psi_1^\dagger(\tau) H_{12} \mathcal{G}(\tau - \tau') H_{21} \Psi(\tau') \right\}, \quad (\text{S8})$$

where the constant  $\mathcal{C} \equiv \int \mathcal{D}\Psi_2 \mathcal{D}\Psi_2^\dagger \exp \left\{ \int d\tau \Psi_2^\dagger \mathcal{G}^{-1} \Psi_2 \right\}$ . Inserting the last result into Eq. (S2), we obtain

$$\mathcal{Z} = \int \mathcal{D}\Psi_1 \mathcal{D}\Psi_1^\dagger \exp \left\{ - \int d\tau \int d\tau' \Psi_1^\dagger(\tau) \{ \delta(\tau - \tau') (\partial_\tau + H_{11}) + H_{12} \mathcal{G}(\tau - \tau') H_{21} \} \Psi_1(\tau') \right\} \quad (\text{S9})$$

$$= \int \mathcal{D}\Psi_1 \mathcal{D}\Psi_1^\dagger \exp \left\{ - \int d\omega \Psi_1^\dagger(i\omega) \{ i\omega + H_{11} + H_{12} \mathcal{G}(i\omega) H_{21} \} \Psi_1(i\omega) \right\}. \quad (\text{S10})$$

We consider topology defined in terms of on-shell quasiparticles with the infinite lifetime, both for the parent topological crystal and the PTB. Therefore, we set  $i\omega \rightarrow 0$  in the above partition function, which, after using the form of the Green's function in Eq. (S5), yields

$$H_{\text{PTB}} = H_{11} - H_{12} H_{22}^{-1} H_{21}, \quad (\text{S11})$$

with the minus arising from the form of the Green's function  $\mathcal{G}(i\omega = 0)$ . This is exactly the form of Eq. (1) in the main text. Therefore, for on-shell quasiparticles the Hamiltonian in the parent topological crystal [ $H_{\text{parent}}$  in Eq. (S1)] and PTBs [ $H_{\text{PTB}}$  in Eq. (S11)] are Hermitian, and both operators possess real energy eigenvalue spectra.

We therefore obtain that the brane Hamiltonian is a Schur complement with respect to the Hamiltonian  $H_{22}$ , which acts in the Hilbert space of the states outside the brane, and thus we can write

$$H_{\text{PTB}} \equiv H_{\text{parent}} / H_{22}. \quad (\text{S12})$$

This relation is well defined in the usual sense of the matrix inversion when  $H_{22}$  is invertible. In practise, this is always the case as we are dealing with the finite size systems.

Let us now explore the relationship between the gap structure of the  $H_{\text{PTB}}$  and  $H_{\text{parent}}$ . As shown in Ref. [1], when  $H_{22}$  is non-singular, the corresponding determinants are related by

$$\det H_{\text{parent}} = \det H_{22} \det H_{\text{PTB}}. \quad (\text{S13})$$

Therefore, we can conclude that when the brane Hamiltonian,  $H_{\text{PTB}}$  is gapped, the same is true for the parent state. Now, to consider the case when the matrix  $H_{22}$  is singular, we recall that in physically relevant situations, the zero energy states, which are responsible for the non-invertibility, are *isolated* in the spectrum. The scaling of the gap at the nodal point (either in the bulk or at the system's boundary) with the system size is  $\sim 1/L$ , where  $L$  is the linear system size, with the nodal point pinned at zero energy only in the thermodynamic limit. The relation in Eq. (S13) can therefore be applied for any finite system size. Since this scaling is a continuous function of the system size and the zero modes are isolated, we conjecture that the existence of the zero modes on the lower-dimensional brane implies that the zero modes are also hosted by the parent system. The opposite, however, does not hold, as can be seen from the example of a dislocation defect, which in spite of featuring zero mode in the parent state does not necessary feature the zero energy states on the brane. The latter is true only when the projection of the dislocation core lies within the lower-dimensional brane.

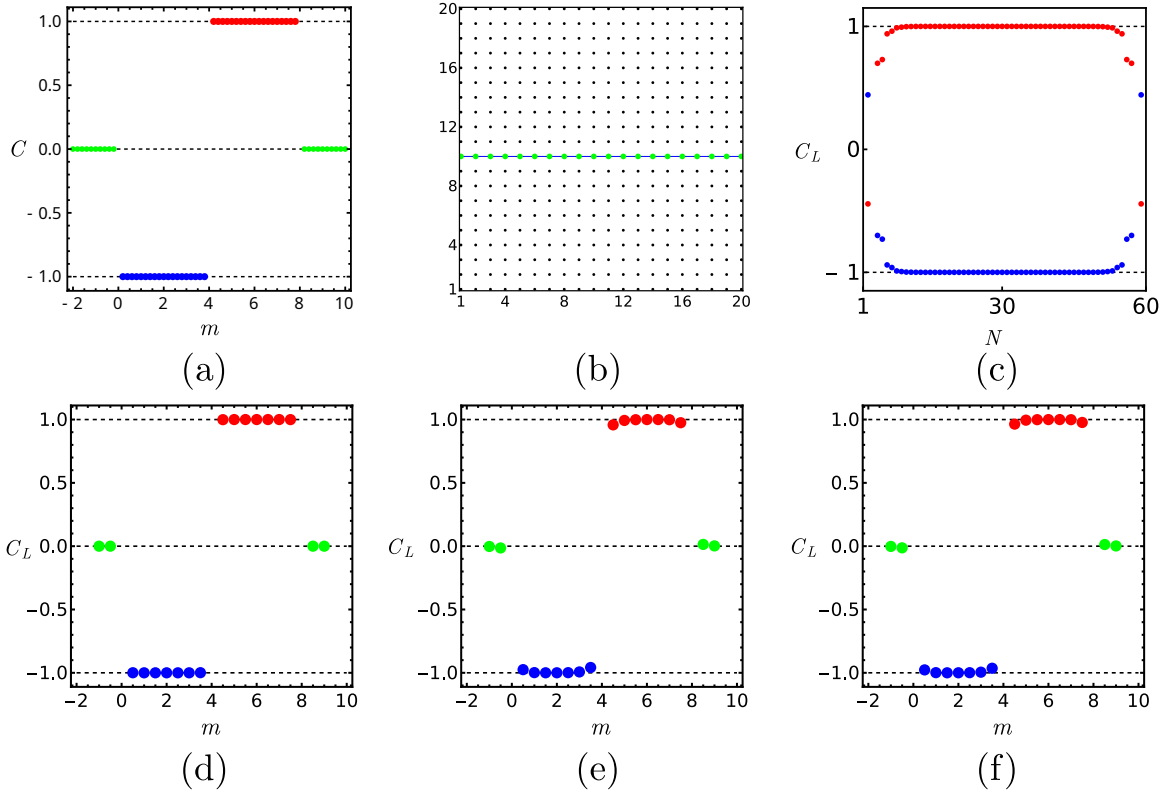

Supplementary Figure 1: (a) Chern Number [ $C$ , defined in Eq.(S15)] of the Hamiltonian in Eq.(S14). The green, blue and red stand for the trivial insulator, the  $\Gamma$  phase, and the  $M$  phase, respectively. Both  $\Gamma$  and  $M$  phases correspond to topological insulators with Chern number  $C = -1$  and  $1$ , respectively. (b) A schematic representation of the computation of the local Chern number [ $C_L$ , defined in Eq. (S19)] along a line containing the green sites, falling at the middle (in the  $y$  direction) of a  $20 \times 20$  square lattice. (c) Variation of  $C_L$  on such a line on a  $60 \times 60$  square lattice for  $m/t_0 = 6$  (red dots) and  $6$  (blue dots), showing that in the bulk of the system  $C_L$  matches with  $C$  [panel (a)]. (d) Variation of  $C_L$  computed at the center of the line shown in panel (b) with  $m/t_0$  of a  $60 \times 60$  square lattice, showing agreement with panel (a). Variation of  $C_L$  with  $m/t_0$  computed at the center of the line, defined by  $y_{\text{mid}} = (y_u + y_d)/2$ , residing within the PTBs, inclined at (e) rational and (f) irrational slope in the parent square lattice, showing agreement with panel (a) and (d). The slight deviation of  $C_L$  from perfect quantization (within numerical accuracy) near the band gap closing is solely due to finite size effects. Therefore, the local Chern number  $C_L$  is a bonafide topological invariant for PTBs. Here the PTBs are constructed from a parent square lattice of linear dimension  $L = 100$  in both  $x$  and  $y$  directions, with  $x_u = 22$  and  $x_d = 12$ , such that they contain (e) 10.3% and (f) 10.6% of the sites of the parent crystal. We here set  $t = 2$  and  $t_0 = 1$ . The rest of the details are same as in Figs. 1 and 5 of the main text.

## Supplementary Note 2. CHERN NUMBER OF MODEL IN EQ.(3) OF THE MAIN TEXT

In this section of the Supplementary Information we discuss the following. (a) Hamiltonian for the spinless Bernevig-Hughes-Zhang model, featuring topological Chern insulators and the explicit definition of the Chern number ( $C$ ). (b) Implementation of the spinless Bernevig-Hughes-Zhang model on a square lattice.

### A. Chern insulator and Chern number

We consider the spinless Bernevig-Hughes-Zhang model for 2D insulators (both topological and trivial or normal) [2]. It reads as

$$H = t \sum_{j=x,y} \sin(k_j a) \tau_j - \left[ m - 2t_0 \sum_{j=x,y} [1 - \cos(k_j a)] \right] \tau_z \equiv \mathbf{d}(\mathbf{k}) \cdot \boldsymbol{\tau}. \quad (\text{S14})$$

The Chern number of this model, defined as

$$C = \frac{1}{4\pi} \int_{\text{BZ}} d^2\mathbf{k} \left( \partial_{k_x} \hat{\mathbf{d}}(\mathbf{k}) \times \partial_{k_y} \hat{\mathbf{d}}(\mathbf{k}) \right) \cdot \hat{\mathbf{d}}(\mathbf{k}), \quad (\text{S15})$$

where  $\hat{\mathbf{d}}(\mathbf{k}) = \mathbf{d}(\mathbf{k})/|\mathbf{d}(\mathbf{k})|$ . The Chern number is plotted in Supplementary Figure 1 as a function of  $m$ . Throughout we have set  $t = t_0 = 1$ , and the lattice spacing  $a = 1$ . The momentum integral is performed over the first Brillouin zone. For  $0 < m/t_0 < 4$  ( $4 < m/t_0 < 8$ ), the system exhibits the  $\Gamma$  phase ( $M$  phase), where the band inversion occurs at the  $\Gamma = (0, 0)$  point ( $M = (\pi, \pi)$  point) in the Brillouin Zone. For other values of  $m/t_0$ , the system is a trivial or normal insulator. The Chern number for the topological insulator in the  $\Gamma$  and  $M$  phases are respectively  $C = -1$  and  $C = +1$ .

### B. Real space version of the spinless Bernevig-Hughes-Zhang Hamiltonian

The above model [Eq. (S14)] translates into the following real space hopping Hamiltonian after performing the Fourier transformation

$$\begin{aligned} \hat{h}_{\text{real}} = & \sum_{n_x=1}^{L_x} \sum_{n_y=1}^{L_y} (2t_0 - m) c_{n_x, n_y}^\dagger c_{n_x, n_y} \otimes \tau_z \\ & - \left[ \left\{ \sum_{n_x=1}^{L_x-1} \sum_{n_y=1}^{L_y} c_{n_x, n_y}^\dagger c_{n_x+1, n_y} \otimes \left( t_0 \tau_z + \frac{it\tau_x}{2} \right) + \sum_{n_x=1}^{L_x} \sum_{n_y=1}^{L_y-1} c_{n_x, n_y}^\dagger c_{n_x, n_y+1} \otimes \left( t_0 \tau_z + \frac{it\tau_y}{2} \right) \right\} + H.C. \right]. \end{aligned} \quad (\text{S16})$$

Here,  $L_x$  ( $L_y$ ) represents the number of sites in the  $x$  ( $y$ ) direction. After implementing the above tight-binding model on a square lattice, we identify the sites belonging to the projected brane and the ones falling outside it [see Fig. 1 of the main text]. Subsequently, we compute  $H_{\text{PTB}}$  following the prescription discussed in Sec. Supplementary Note 1 [Eq. (S11)] and numerically diagonalize  $H_{\text{PTB}}$  to study its topological features, such as the endpoint near zero energy modes [see Fig. 2 of the main text].

### C. Local Chern number ( $C_L$ ) on a square lattice

In this section, we show the computation of the local Chern number for square lattice spinless Bernevig-Hughes-Zhang model, introduced in Eq. (S14). We follow the prescription from Ref. [3]. For the sake of concreteness, here we focus on a half-filled system, such that all the states at negative energies are completely filled, while the ones at positive energies are left empty. Notice that due to finite size effect even the edge modes are placed at finite but *small* positive energies in systems with open boundary condition. Accordingly, we define a projector ( $P$ ) and its complement ( $Q$ ) respectively in the following way

$$P = \sum_{E_n < 0} |\psi_n\rangle \langle \psi_n|, \quad \text{and} \quad Q = \mathbf{I} - P, \quad (\text{S17})$$

where  $\mathbf{I}$  is an identity matrix. Here  $|\psi_n\rangle$  is the eigenstate of  $\hat{h}_{\text{real}}$  [see Eq. (S16)] on a square lattice with energy  $E_n$ . Then the local Chern operator or matrix is defined as

$$\hat{C}_L = -4\pi \text{Im} \left[ P \hat{X} Q \hat{Y} P \right], \quad (\text{S18})$$

where  $\hat{X}$  and  $\hat{Y}$  are the position operators in the  $x$  and  $y$  directions, respectively. Since these two operators are not periodic, our results are qualitatively insensitive to whether we impose periodic or open boundary condition. The local Chern number at a given site located on a two-dimensional square lattice at position  $\mathbf{r}$  can then be computed from  $\hat{C}_L$  in the following way

$$C_L(\mathbf{r}) = \sum_{j=1}^2 \langle \mathbf{r}_j | \hat{C}_L | \mathbf{r}_j \rangle. \quad (\text{S19})$$

Here the summation over  $j = 1, 2$  accounts for two sublattice or orbital degrees of freedom over which the vector Pauli matrix  $\boldsymbol{\tau}$  operates on, and  $|\mathbf{r}_j\rangle$  is the state vector of the site located at  $\mathbf{r}$  with orbital  $j$ . We choose a set of

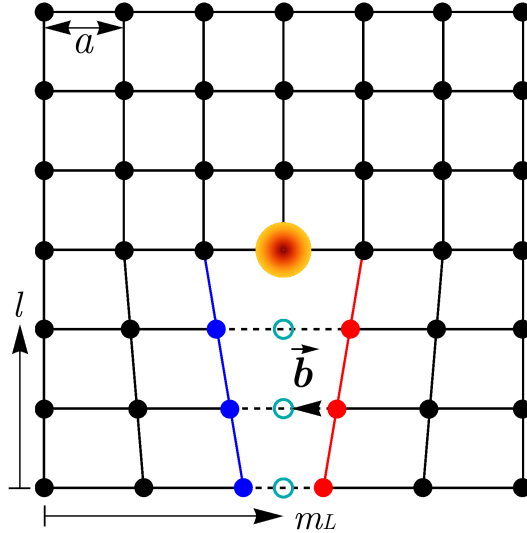

Supplementary Figure 2: Construction of a single edge dislocation through Volterra cut-and-glue procedure on a parent square lattice by removing a line of atoms (open cyan circles), ending at the center or core of the dislocation (orange circle) and subsequently reconnecting (represented by the dashed lines) the sites (red and blue dots) living on the edges (red and blue lines) across it. The corresponding Burgers vector is  $\mathbf{b} = a\mathbf{e}_x$ . In the main text, we have used  $L_x = 61$ ,  $L_y = 60$ ,  $m_L = 31$ , and  $l = 30$ .

sites shown in green color in Supplementary Figure 1(b) and the variation of the local Chern number along that line for specific values of  $m/t_0$  are shown in Supplementary Figure 1(c). We find that on the sites, residing in the bulk of the system, the local Chern number is quantized to the values also predicted from Eq. (S15). By taking the value of  $C_L$  at the site residing at the center of this line, we show the variation of  $C_L$  as a function of  $m/t_0$  in Supplementary Figure 1(d), which agrees with the one obtained from the Chern number  $C$  computed from Eq. (S15) and shown in Supplementary Figure 1(a).

#### D. Local Chern number of projected topological branes

In this section we discuss the key steps of computing the local Chern number on one-dimensional PTBs, inclined at a rational or an irrational slope inside the parent square lattice. In the first step, we compute the effective Hamiltonian  $H_{\text{PTB}}$  [Eq. (S11)] for the PTBs, following the prescription from Sec. Supplementary Note 1. Subsequently, we construct the local Chern operator or matrix defined in Eq. (S18) for the PTB with  $\hat{X}$  and  $\hat{Y}$  restricted within the PTBs. In the final step, we compute the local Chern number following Eq. (S19) on the sites (blue sites) falling within the PTBs and residing in between two confining red lines (green line, defined by  $y_{\text{mid}} = (y_u + y_d)/2$ ), shown in Figs. 5(a) and 5(c) of the main text, with their position  $\mathbf{r}$  on the parent square lattice. The variation of the local Chern number on such a line for specific choices of  $m/t_0$  are shown in Figs. 5(b) and 5(d) of the main text. The variations of  $C_L$  on a site residing at the center of the green line on PTBs, inclined at a rational or an irrational slope in the square lattice, with  $m/t_0$  are shown in Supplementary Figure 1(e) and Supplementary Figure 1(f) of this SI, which are identical to that on the parent square lattice, shown in Supplementary Figure 1(d).

#### Supplementary Note 3. REAL SPACE HAMILTONIAN WITH A SINGLE EDGE DISLOCATION

To create a single dislocation in a lattice, we remove a line of sites along  $x = m_L$ , from  $y = 1$  to  $y = l$ . For  $y < l + 1$ , we recreate the hopping elements between the sites at  $x = m_L - 1$  and  $x = m_L + 1$ , so that they behave as adjacent sites. The site at  $x = m_L, y = l + 1$  is the dislocation center. For  $y \geq l + 1$ , the number of lattice sites in the  $x$  direction is  $L_x$  for each discrete value of  $y$ , while for  $y < l$ , there are  $L_x - 1$  number of sites in the  $x$  direction for each  $y$ . See Supplementary Figure 2.

The Hamiltonian [see Eq. (S14)] when implemented on a square lattice, containing a single edge dislocation, takes

the form

$$\begin{aligned}
\hat{h}_{\text{dislocation}} = & \sum_{\text{all sites}} \sum (2t_0 - m) c_{n_x, n_y}^\dagger c_{n_x, n_y} \otimes \tau_z \\
& - \left[ \sum_{n_x=1}^{m_L-2} \sum_{n_y=1}^l c_{n_x, n_y}^\dagger c_{n_x+1, n_y} \otimes \left( t_0 \tau_z + \frac{it\tau_x}{2} \right) + \sum_{n_y=1}^l c_{m_L-1, n_y}^\dagger c_{m_L+1, n_y} \otimes \left( t_0 \tau_z + \frac{it\tau_x}{2} \right) \right. \\
& + \sum_{n_x=m_L+1}^{L_x-1} \sum_{n_y=1}^l c_{n_x, n_y}^\dagger c_{n_x+1, n_y} \otimes \left( t_0 \tau_z + \frac{it\tau_x}{2} \right) + \sum_{n_x=1}^{L_x-1} \sum_{n_y=l+1}^{L_y} c_{n_x, n_y}^\dagger c_{n_x+1, n_y} \otimes \left( t_0 \tau_z + \frac{it\tau_x}{2} \right) \Bigg] + H.C. \\
& - \left[ \sum_{n_x=1}^{m_L-1} \sum_{n_y=1}^{L_y-1} c_{n_x, n_y}^\dagger c_{n_x, n_y+1} \otimes \left( t_0 \tau_z + \frac{it\tau_y}{2} \right) + \sum_{n_y=l+1}^{L_y-1} c_{m_L, n_y}^\dagger c_{m_L, n_y+1} \otimes \left( t_0 \tau_z + \frac{it\tau_y}{2} \right) \right. \\
& + \sum_{n_x=m_L+1}^{L_x} \sum_{n_y=1}^{L_y-1} c_{n_x, n_y}^\dagger c_{n_x, n_y+1} \otimes \left( t_0 \tau_z + \frac{it\tau_y}{2} \right) \Bigg] + H.C. \quad (S20)
\end{aligned}$$

Upon implementing the above Hamiltonian on a parent square lattice, we once again identify the sites belong to and falling outside the projected brane, and subsequently construct  $H_{\text{PTB}}$  following the prescription from Sec. Supplementary Note 1 with the core of the edge dislocation always falling within such brane. See Figs. 3 and 4 of the main text.

#### Supplementary Note 4. 3D WEYL SEMIMETALS: LATTICE MODEL, LANDAU LEVELS, AND CHIRAL ANOMALY

A three dimensional (3D) Weyl semimetal can be realized by stacking 2D Chern insulators in a translationally invariant fashion. This procedure leads to the following Hamiltonian

$$H_{\text{weak}} = H + t_z \cos(k_z a) \tau_z \equiv t \sum_{j=x,y} \sin(k_j a) \tau_j - \left[ m - 2t_0 \sum_{j=x,y} [1 - \cos(k_j a)] \right] \tau_z + t_z \cos(k_z a) \tau_z. \quad (S21)$$

The real space representation of this Hamiltonian (under open boundary condition) is

$$\begin{aligned}
\hat{h}_{\text{weak}} = & \sum_{n_x=1}^{L_x} \sum_{n_y=1}^{L_y} \sum_{n_z=1}^{L_z} (2t_0 - m) c_{n_x, n_y, n_z}^\dagger c_{n_x, n_y, n_z} \otimes \tau_z - \left[ \sum_{n_x=1}^{L_x-1} \sum_{n_y=1}^{L_y} \sum_{n_z=1}^{L_z} c_{n_x, n_y, n_z}^\dagger c_{n_x+1, n_y, n_z} \otimes \left( t_0 \tau_z + \frac{it\tau_x}{2} \right) \right. \\
& + \sum_{n_x=1}^{L_x} \sum_{n_y=1}^{L_y-1} \sum_{n_z=1}^{L_z} c_{n_x, n_y, n_z}^\dagger c_{n_x, n_y+1, n_z} \otimes \left( t_0 \tau_z + \frac{it\tau_y}{2} \right) \Bigg] + H.C. \\
& + \frac{t_z}{2} \left[ \sum_{n_x=1}^{L_x} \sum_{n_y=1}^{L_y} \sum_{n_z=1}^{L_z-1} c_{n_x, n_y, n_z}^\dagger c_{n_x, n_y, n_z+1} \otimes \tau_z + H.C. \right]. \quad (S22)
\end{aligned}$$

Next we compute the band structure of this model featuring a single pair of Weyl nodes (depending on the relative strenght of  $t$ ,  $t_0$ ,  $t_z$  and  $m$ ), Landau levels in the presence of uniform magnetic field applied in the  $z$  direction. Finally, we introduce a singular magnetic flux tube to test the validity of the predictions for the chiral anomaly in case of the 3D Weyl semimetal.

Subsequently, these analyses are repeated for the projected Weyl brane in two dimensions. During this procedure we construct the projected Hamiltonian within the brane by integrating out the sites falling outside it (according to Eq. (S11)), which otherwise lie within the  $xy$  plane. No projection is performed in the  $z$  direction.

#### A. Band structure of three-dimensional (3D) Weyl semimetals (WSMs)

In Supplementary Figure 3(a) we display the band structure of the Hamiltonian  $H_{\text{weak}}$  for  $t = 2t_0 = t_z = 1$  and  $m = 4$ . For this choice of the parameters, the system supports a single pair of Weyl nodes at  $\mathbf{k} = (1, 1, \pm 1/2)\pi$

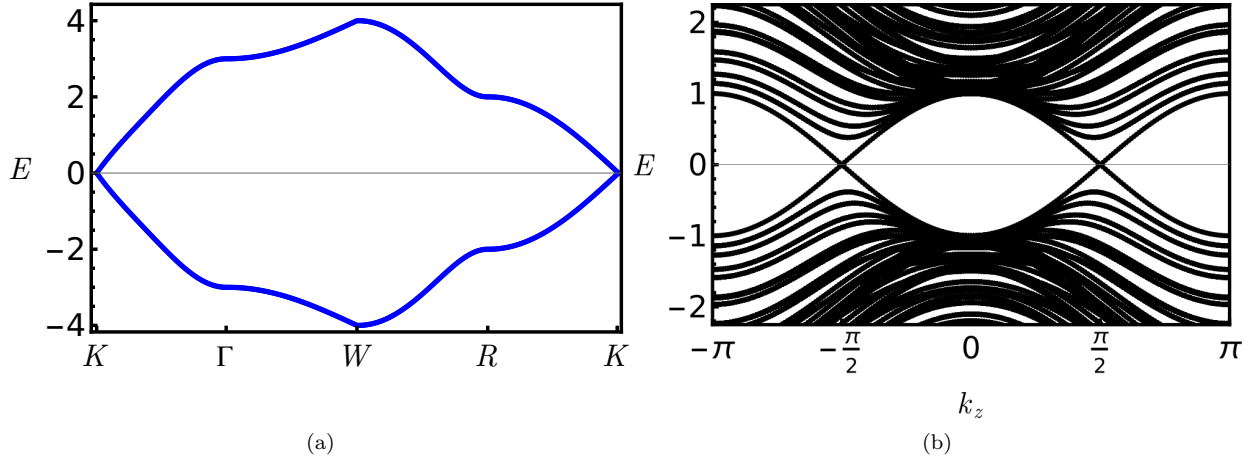

Supplementary Figure 3: (a) Band structure of the Hamiltonian  $H_{\text{weak}}$  [Eq. (S21)] in the reciprocal space for a parent 3D Weyl semimetal. Here we follow a path along  $K \rightarrow \Gamma \rightarrow W \rightarrow R \rightarrow K$  in the 3D Brillouin zone. The locations of various points therein are  $K = (\pi, \pi, \frac{\pi}{2})$ ,  $\Gamma = (0, 0, 0)$ ,  $W = (0, 0, \frac{\pi}{2})$ ,  $R = (\pi, 0, \frac{\pi}{2})$  [with lattice spacing  $a = 1$ ]. (b) Band structure of the parent Weyl semimetal as a function of  $k_z$ , computed after implementing  $H_{\text{weak}}$  on a square lattice in the  $xy$  plane with periodic boundary condition, keeping  $k_z$  as a good quantum number. In both (a) and (b), we set  $t = 2t_0 = t_z = 1, m = 4$ . Therefore, a single pair of Weyl nodes appear at momentum  $\mathbf{k} = (\pi, \pi, \pm \frac{\pi}{2})$ .

of the 3D Brillouin zone. In addition, we ensure that around these two points the energy dispersion scales linearly with  $k_z$ . Therefore, we also plot the energy spectra as a function of  $k_z$  (a good quantum number) by implementing the hopping terms, depending on  $k_x$  and  $k_y$  on a real space square lattice and subsequently imposing the periodic boundary condition in the  $x$  and  $y$  directions. Supplementary Figure 3(b) shows that indeed the energy scales linearly with  $k_z$  around two Weyl nodes at  $k_z = \pm\pi/2$ .

Following the prescription of constructing  $H_{\text{PTB}}$  we plot the band structure of projected Weyl brane with  $k_z$  as good quantum number. We find that the Weyl brane also supports a single pair of Weyl nodes exactly at  $k_z = \pm\pi/2$ . See Figs. 6(a) and 6(d) of the main text.

### B. Fermi Arc surface states of 3D Weyl semimetals

The hallmark of 3D Weyl semimetal is the Fermi arc surface states, encoding the bulk-boundary correspondence. It can be constructed in the following way. Recall that a Weyl semimetal is built by stacking layers of Chern insulators between two Weyl nodes in the momentum space. Therefore, each layer of such Chern insulator supports zero energy edge modes, however, only between two Weyl nodes. A collection of such zero energy edge modes ultimately constitutes the Fermi arc connecting two Weyl nodes. Our numerical results on Fermi arc states are shown in Supplementary Figure 4.

First we show the Fermi arc states in a mixed Bloch-Wannier representation, in which we numerically diagonalize  $H_{\text{weak}}$  with real space hopping Hamiltonian in the  $xy$  plane, while treating  $k_z$  as a good quantum number. The result is shown in Supplementary Figure 4(a). Indeed we find that zero energy modes exist only in between two Weyl nodes at  $k_z = \pm\pi/2$ . For each value of  $k_z$  in between the Weyl nodes the zero energy edge mode occupies the  $xy$  plane. A collection of such edge modes give rise to the ribbon-like Fermi arc state in a 3D Weyl semimetal.

Next we implement  $H_{\text{weak}}$  in a 3D cubic lattice. The numerical diagonalization then reveals ribbon-like Fermi arc surface states occupying the  $xz$  and  $yz$  planes. The results are shown in Supplementary Figure 4(b).

When we construct the projected Weyl brane, it also contains the signature of the Fermi arc surface states which we confirm with the above two geometries. Namely, when we treat  $k_z$  as a good quantum number, and for its each value construct  $H_{\text{PTB}}$ , the Fermi arcs are observed for  $|k_z| \leq \pi/2$ . See Figs. 6(b) and (e) of the main text. On the other hand, when we construct  $H_{\text{PTB}}$  from a hopping Hamiltonian of the parent 3D Weyl semimetal, the Fermi arc states are extended in the  $z$  direction. See Figs. 6(c) and (f) of the main manuscript.

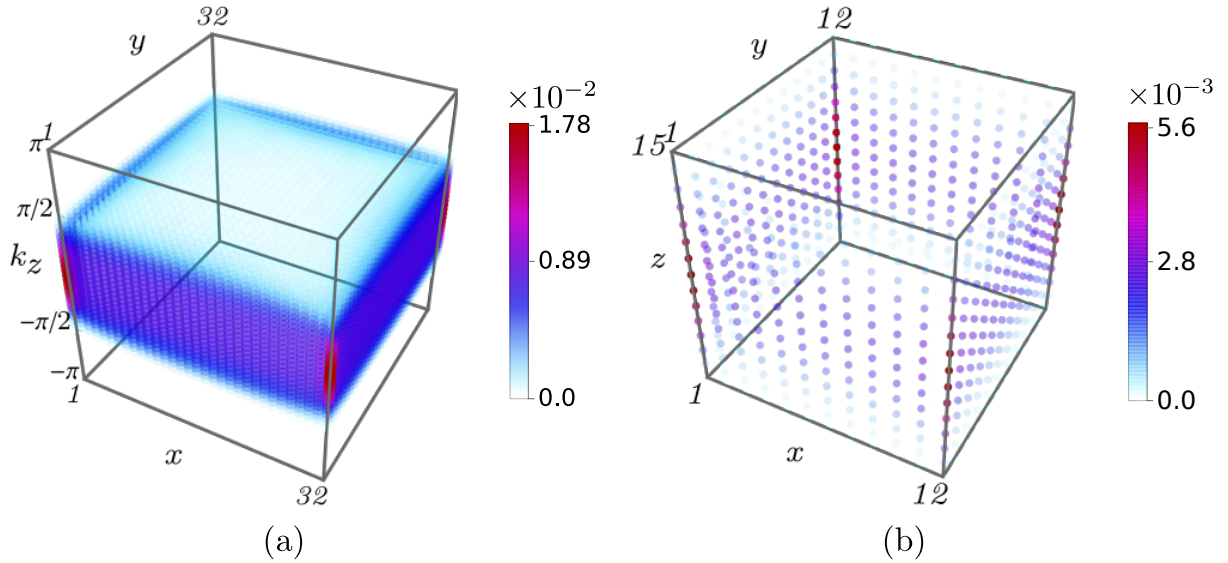

Supplementary Figure 4: (a) Zero energy Fermi arc states in the mixed Bloch-Wannier representation, obtained by numerically diagonalizing  $H_{\text{weak}}$  by treating  $k_z$  as a good quantum number. The Fermi arc states only occupy the regime in between two Weyl nodes located at  $k_z = \pm\pi/2$ , and the  $k_z - x$  and  $k_z - y$  planes. Here we impose open boundary condition in the  $x$  and  $y$  directions. (b) Fermi arc states on a  $12 \times 12 \times 15$  3D lattice with open boundary conditions in all three directions. The Fermi arc surface states in this geometry occupy the  $xz$  and  $yz$  planes. In both cases, we set  $m = 4$ , and  $t = 2t_0 = t_z = 1$ . Compare Fig. 5 of the main text.

### C. 3D Landau levels with explicit form of Peierls factors

The orbital effects of the magnetic field is taken into account via the Peierls substitution, in which momentum  $\mathbf{p} \rightarrow \mathbf{p} - e\mathbf{A}$ , where  $\mathbf{A}$  is the magnetic vector potential. Suppose, before applying the magnetic field, the hopping element between sites  $(n_x, n_y)$  and  $(n_x + 1, n_y)$  was equal to 1. In the presence of the magnetic field, it is replaced by  $e^{-ieA_x a}$ , where  $a$  is the lattice constant. Similarly, the hopping elements between sites  $(n_x, n_y)$  and  $(n_x, n_y + 1)$  acquires a factor of  $e^{-ieA_y a}$ . We choose an appropriate gauge, and modify the hopping elements in this manner. The Landau levels of the parent system are shown in Supplementary Figure 5.

For the calculation of Landau levels (LLs) for a magnetic field  $\mathbf{B} = \frac{1}{L_y}\hat{z}$ , we work with the Landau gauge,  $\mathbf{A} = (-By, 0, 0)$ . We work with atomic units,  $\hbar = e = 1$ , and set the lattice constant  $a = 1$ . Here  $L_y$  is the linear dimension of the system in the  $y$  direction. Therefore, the mixed Bloch-Wannier representation of the Hamiltonian is,

$$\begin{aligned} \hat{h}_{\text{LL}}(B, k_z) = & \sum_{n_x=1}^{L_x} \sum_{n_y=1}^{L_y} (2t_0 - m + t_z \cos k_z) c_{n_x, n_y}^\dagger c_{n_x, n_y} \otimes \tau_z - \left[ \sum_{n_x=1}^{L_x-1} \sum_{n_y=1}^{L_y} c_{n_x, n_y}^\dagger c_{n_x+1, n_y} \otimes e^{-iBn_y} \left( t_0 \tau_z + \frac{it\tau_x}{2} \right) \right. \\ & \left. + \sum_{n_x=1}^{L_x} \sum_{n_y=1}^{L_y-1} c_{n_x, n_y}^\dagger c_{n_x, n_y+1} \otimes \left( t_0 \tau_z + \frac{it\tau_y}{2} \right) \right] + H.C. \end{aligned} \quad (\text{S23})$$

The Landau level spectra of the above model is computed with  $k_z$  as a good quantum number, as the translational symmetry in the direction of external magnetic field remains preserved, and with periodic (open) boundary condition in the  $x$  ( $y$ ) direction. The results are shown in Supplementary Figure 5, displaying chiral zeroth Landau level crossing the zero energy at the Weyl nodes at  $k_z = \pm\pi/2$ . While computing the Landau levels for the projected Weyl brane, we project the hopping elements of the above model within the  $xy$  plane onto the brane, but treat  $k_z$  as good quantum number. Remarkably, the Weyl branes also support topological protected chiral zeroth Landau levels that also cross the zero energy at  $k_z = \pm\pi/2$ . See Figs. 7(a) and (c) of the main text.

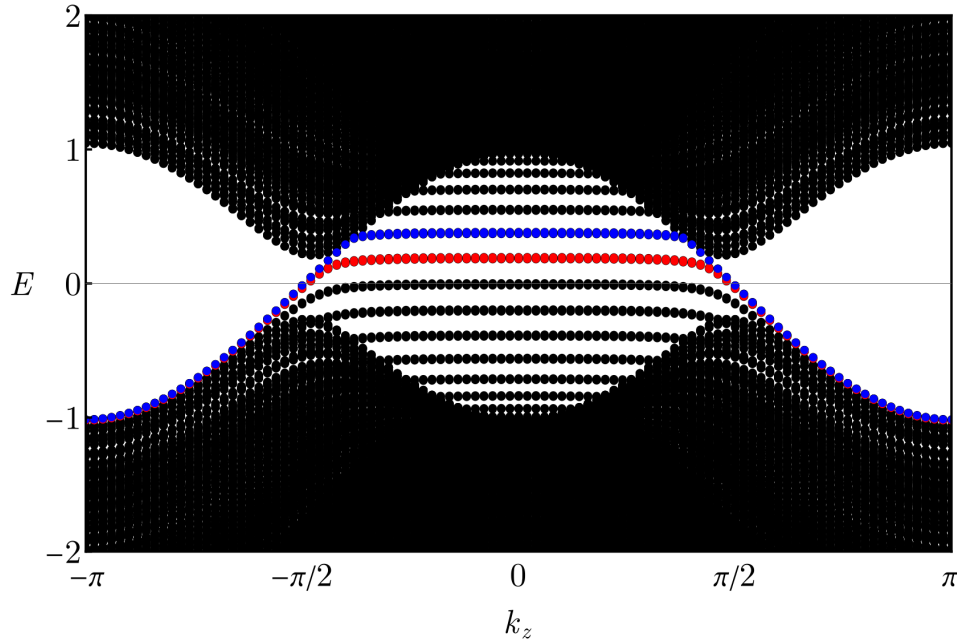

Supplementary Figure 5: Landau Levels in parent crystal of dimension  $L_x = L_y = 32$  in both  $x$  and  $y$  directions with  $k_z$  as a good quantum number, for parameters  $t = 2t_0 = t_z = 1$ ,  $m = 4$  and  $\mathbf{B} = \frac{1}{L_y}\hat{z}$ . We chose the Landau gauge  $\mathbf{A} = (-By, 0, 0)$ , and employed periodic boundary conditions along  $x$  direction, and open boundary conditions along  $y$  direction. Each of the red and blue levels have a two-fold degeneracy, and they correspond to the chiral zeroth Landau level, crossing the zero energy at  $k_z = \pm\pi/2$ , exactly where the Weyl nodes are located.

#### D. Singular flux configuration and charge accumulation due to chiral anomaly

Here we show how to introduce a magnetic field that is non-zero only on a singular tube at the center of the lattice and points in the  $z$  direction. We choose the corresponding vector potential to be

$$\mathbf{A} = Ba^2\Theta\left(x - \frac{L_x}{2} - \frac{1}{2}\right)\delta\left(y - \frac{L_y}{2} - \frac{1}{2}\right)\hat{y}. \quad (\text{S24})$$

Here  $\Theta(x)$  is the Heaviside step function, and  $\delta(x)$  is the Dirac delta function. The magnetic flux passing through the central square is  $\Phi = Ba^2$ .

On a lattice, the delta function can only be resolved up to the length scale of the lattice constant  $a$ , and the vector potential non-zero on the right half of the parent crystal, only between the sites at  $y = \frac{L_y}{2}$  and  $y = \frac{L_y}{2} + 1$ . It is represented by the purple arrows in Supplementary Figure 6(a) and (b). The lattice plaquette through which a singular magnetic flux pierces the system is shown by blue box in this figure. Notice that such plaquette is always enclosed by the projected topological brane, irrespective of whether it displays emergent crystalline or quasicrystalline order.

Considering  $k_z$  to be a good quantum number, the Bloch-Wannier representation of the Hamiltonian in the presence of such a singular magnetic flux tube (FT) is

$$\begin{aligned} \hat{h}_{\text{FT}}(\Phi, k_z) = & \sum_{n_x=1}^{L_x} \sum_{n_y=1}^{L_y} (2t_0 - m) c_{n_x, n_y}^\dagger c_{n_x, n_y} \otimes \tau_z - \left[ \sum_{n_x=1}^{L_x-1} \sum_{n_y=1}^{L_y} c_{n_x, n_y}^\dagger c_{n_x+1, n_y} \otimes \left( t_0 \tau_z + \frac{it\tau_x}{2} \right) + H.C. \right] \\ & - \left[ \sum_{n_x=1}^{L_x} \sum_{n_y=1}^{L_y/2-1} c_{n_x, n_y}^\dagger c_{n_x, n_y+1} \otimes \left( t_0 \tau_z + \frac{it\tau_y}{2} \right) + H.C. \right] - \left[ \sum_{n_x=1}^{L_x/2} c_{n_x, L_y/2}^\dagger c_{n_x, L_y/2+1} \otimes \left( t_0 \tau_z + \frac{it\tau_y}{2} \right) + H.C. \right] \\ & - \left[ \sum_{n_x=L_x/2+1}^{L_x} c_{n_x, L_y/2}^\dagger c_{n_x, L_y/2+1} \otimes e^{i\Phi} \left( t_0 \tau_z + \frac{it\tau_y}{2} \right) + H.C. \right] \end{aligned}$$

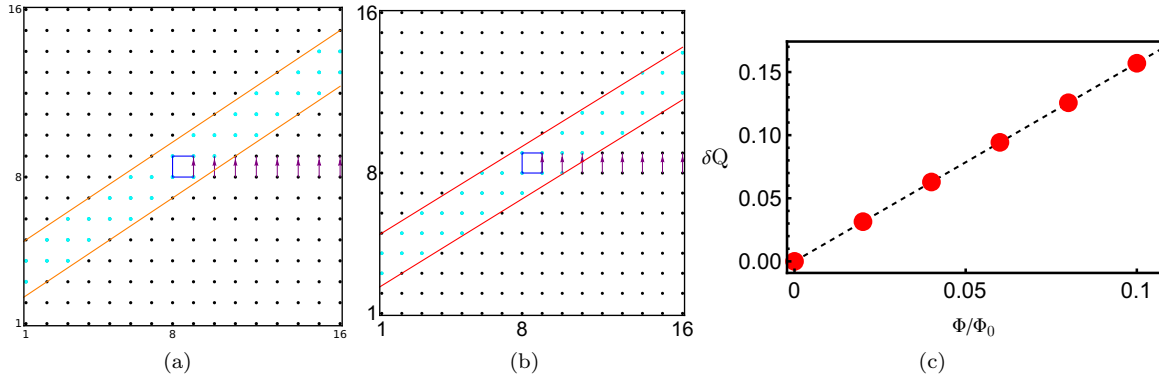

Supplementary Figure 6: Illustration of flux tube (blue square in the center) passing through (a) Rational and (b) Irrational topological branes (cyan sites), respectively displaying emergent crystalline and quasicrystalline orders, between the red lines defined by  $y_i = S(x - \tilde{x}_i) + x_i$  for  $i = u$  and  $d$ , with  $x_u > x_d$ ,  $\tilde{x}_u = 1$ ,  $x_u = 5$ , and  $\tilde{x}_d = 2$ ,  $x_d = 3$ . Here  $x$  represents the horizontal coordinate of the red lines. In (a)  $S = 2/3$  and in (b)  $S = \varphi^{-1}$ , where  $\varphi = (1 + \sqrt{5})/2$  is the golden ratio. The vector potential, wherever non-zero, is shown by a purple line, and its direction is denoted by the arrowheads. (c) Accumulated charge ( $\delta Q$ ) around the flux tube as a function of the magnetic flux  $\Phi$  (measured in units of the flux quanta  $\Phi_0$ ) in a system of linear dimensions  $L_x = L_y = 32$  (this result is for the whole system, and not for the projected brane), with  $k_z$  as a good quantum number. We divide the allowed values of  $k_z \in (-\pi, \pi)$  into 20 points (including the boundaries at  $\pm\pi$ ) at equal intervals, and average the accumulated charge  $\delta Q$  over them. The accumulated charge  $\delta Q$  shows linear dependence on  $\Phi/\Phi_0$  with slope equal to  $\pi/2$  (approximately), showing excellent agreement (with 99.98% accuracy) with the field theoretic prediction, see Sec. Supplementary Note 5.

$$- \left[ \sum_{n_x=1}^{L_x} \sum_{n_y=L_y/2+1}^{L_y-1} c_{n_x, n_y}^\dagger c_{n_x, n_y+1} \otimes \left( t_0 \tau_z + \frac{it\tau_y}{2} \right) + H.C. \right] + t_z \cos k_z \sum_{n_x=1}^{L_x} \sum_{n_y=1}^{L_y} c_{n_x, n_y}^\dagger c_{n_x, n_y} \otimes \tau_z. \quad (\text{S25})$$

The excess charge  $\delta Q$  around the magnetic flux tube is computed by averaging over the one-dimensional Brillouin zone in the  $k_z$  direction, by choosing equally spaced values of  $k_z$  in the interval  $[-\pi, \pi]$ . The results are shown in Supplementary Figure 6(c). While computing the excess charge  $\delta Q$  on Weyl branes, we project the hopping part of the above Hamiltonian in the  $xy$  plane onto the one-dimensional brane, ensuring that the flux tube passes through it, while treating  $k_z$  as a good quantum number. The results are shown in Figs. 6(b) and 6(d) of the main text.

#### Supplementary Note 5. DERIVATION OF EQ.(5) OF MAIN TEXT

The electromagnetic response of a Weyl semimetal constituted by a single pair of Weyl nodes separated by momentum  $2\mathbf{b}$  in the reciprocal space, otherwise placed at the same energy, is described by the action

$$S_\theta = \frac{e^2}{8\pi^2} \int dt d\mathbf{r} \theta(\mathbf{r}, t) \mathbf{E} \cdot \mathbf{B}, \quad (\text{S26})$$

after setting  $\hbar = c = 1$ , with  $\theta(\mathbf{r}, t) = 2\mathbf{b} \cdot \mathbf{r}$ . Notice that  $S_\theta$  bears the signature of the chiral anomaly, manifesting through the anomalous Hall conductivity of a time-reversal symmetry breaking Weyl semimetal, encoded by the equations of motion given by [4–6]

$$\rho = \frac{e^2}{2\pi^2} (\mathbf{b} \cdot \mathbf{B}), \quad \text{and} \quad \mathbf{j} = \frac{e^2}{2\pi^2} (\mathbf{b} \times \mathbf{E}). \quad (\text{S27})$$

Here  $\rho$  and  $\mathbf{j}$  are respectively the induced charge and current densities, related to each other via the Ward identity and  $\mathbf{B}$  is the external magnetic field.

The excess charge density,  $\rho = \frac{e^2}{2\pi^2} (\mathbf{b} \cdot \mathbf{B})$ , where  $2\mathbf{b}$  is the distance between the two Weyl nodes. In the units where the lattice constant is set to unity,  $|\mathbf{b}| = \frac{\pi}{2}$  for the chosen values of the parameters in the tight-binding model for the Weyl semimetal. Then, the total excess charge is,

$$\delta q = \int \rho d^2\mathbf{r} = \frac{e^2}{2\pi^2} b \Phi = \frac{e^2}{4\pi} \Phi. \quad (\text{S28})$$

We measure the excess charge  $\delta Q$  in the units of  $e/\pi$ . Then

$$\delta Q = \frac{\delta q}{e/\pi} = \frac{e}{4} \Phi = \frac{\pi}{2} \frac{\Phi}{2\pi/e} = \frac{\pi}{2} \left( \frac{\Phi}{\Phi_0} \right). \quad (\text{S29})$$

Here  $\Phi_0 = \frac{2\pi\hbar}{e} = \frac{2\pi}{e}$  is the flux quanta. This is identical to Eq. (5) of the main text.

### Supplementary References

---

- [1] Silvester, J. R., Determinants of Block Matrices. *The Mathematical Gazette* **84**, 460 (2000).
- [2] Bernevig, B. A., Hughes, T. L. & Zhang, S.-C., Quantum Spin Hall Effect and Topological Phase Transition in HgTe Quantum Wells, *Science* **314**, 1757 (2006).
- [3] Bianco, R. & Resta, R., Mapping topological order in coordinate space, *Phys. Rev. B* **84**, 241106(R) (2011).
- [4] Zyuzin, A. A. & Burkov, A. A., Topological response in Weyl semimetals and the chiral anomaly, *Phys. Rev. B* **86**, 115133 (2012).
- [5] Vazifeh, M. M. & Franz, M., Electromagnetic Response of Weyl Semimetals, *Phys. Rev. Lett.* **111**, 027201 (2013).
- [6] Dantas, R. M. A., Peña-Benitez, F., Roy, B. & Surówka, P., Non-Abelian anomalies in multi-Weyl semimetals, *Phys. Rev. Research* **2**, 013007 (2020).
